# Supplementary material for: Self-supervised Learning of Interpretable Keypoints from Unlabelled Videos
Source: arXiv:1907.02055 source file (2020-12-23)
Supplement: Supplementary file 3 [file human36m_swap.tex]

\begin{minipage}{\textwidth}
\begin{minipage}[b]{4em}
{\small
\rotatebox{90}{\hspace{-3mm}target image $\bx$}\\
}
\end{minipage}\hspace{-10mm}%
\includegraphics[width=0.117\textwidth]{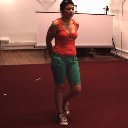}
\includegraphics[width=0.117\textwidth]{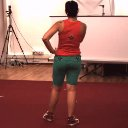}
\includegraphics[width=0.117\textwidth]{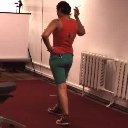}
\includegraphics[width=0.117\textwidth]{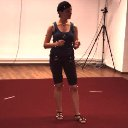}
\includegraphics[width=0.117\textwidth]{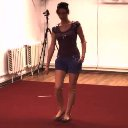}
\includegraphics[width=0.117\textwidth]{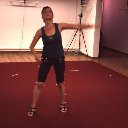}
\includegraphics[width=0.117\textwidth]{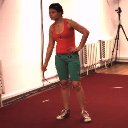}
\includegraphics[width=0.117\textwidth]{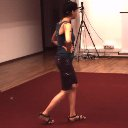}
\\
\begin{minipage}[b]{4em}
{\small
\rotatebox{90}{\hspace{-3mm}style image $\bx'$}\\
}
\end{minipage}\hspace{-10mm}%
\includegraphics[width=0.117\textwidth]{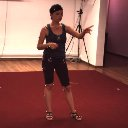}
\includegraphics[width=0.117\textwidth]{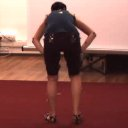}
\includegraphics[width=0.117\textwidth]{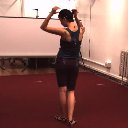}
\includegraphics[width=0.117\textwidth]{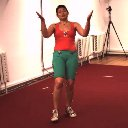}
\includegraphics[width=0.117\textwidth]{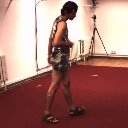}
\includegraphics[width=0.117\textwidth]{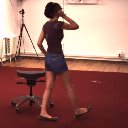}
\includegraphics[width=0.117\textwidth]{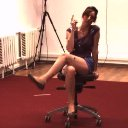}
\includegraphics[width=0.117\textwidth]{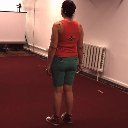}
\\
\begin{minipage}[b]{4em}
{\small
\rotatebox{90}{\hspace{0mm}reconstr. $\hat\bx$}\\
}
\end{minipage}\hspace{-10mm}%
\includegraphics[width=0.117\textwidth]{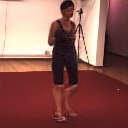}
\includegraphics[width=0.117\textwidth]{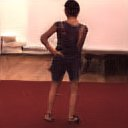}
\includegraphics[width=0.117\textwidth]{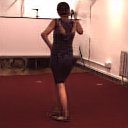}
\includegraphics[width=0.117\textwidth]{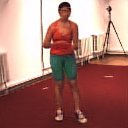}
\includegraphics[width=0.117\textwidth]{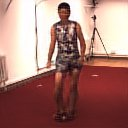}
\includegraphics[width=0.117\textwidth]{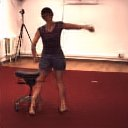}
\includegraphics[width=0.117\textwidth]{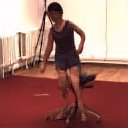}
\includegraphics[width=0.117\textwidth]{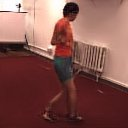}
\\
\end{minipage}
