# Supplementary material for: Self-supervised Learning of Interpretable Keypoints from Unlabelled Videos
Source: arXiv:1907.02055 source file (2020-12-23)
Supplement: Supplementary file 4 [file fig-human36m_swap.tex]

\begin{figure*}[ht]
\centering

\input{texgen/human36m_swap}
\vspace{-4mm}
\input{texgen/face_swap}

\caption{\textbf{Factorization of appearance and geometry.}
We supply different identities for \emph{style} and \emph{{target}} input images. 
\emph{Reconstructed} image inherits appearance from the \emph{style} image and geometry from the \emph{target} image.
{\bf [top]:} human pose samples from Human3.6M.
{\bf [bottom]:} face samples from VoxCeleb2.}
\label{af:swap}
\end{figure*}
