# Supplementary material for: Self-supervised Learning of Interpretable Keypoints from Unlabelled Videos
Source: arXiv:1907.02055 source file (2020-12-23)
Supplement: Supplementary file 5 [file face_move.tex]

\begin{minipage}{\textwidth}
\begin{minipage}[b]{4em}
{\small
\rotatebox{90}{\hspace{0mm}}\\
}
\end{minipage}\hspace{-10mm}%
\hspace{0.1286\textwidth}
\hspace{0.0040\textwidth}
\begin{minipage}[b]{4em}
{\small
\rotatebox{90}{\hspace{-4mm}manip. keypoints}\\
}
\end{minipage}\hspace{-10mm}%
\includegraphics[width=0.129\textwidth]{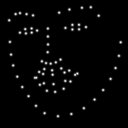}
\includegraphics[width=0.129\textwidth]{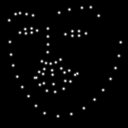}
\includegraphics[width=0.129\textwidth]{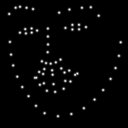}
\includegraphics[width=0.129\textwidth]{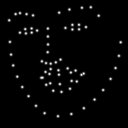}
\includegraphics[width=0.129\textwidth]{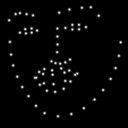}
\includegraphics[width=0.129\textwidth]{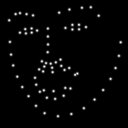}
\\
\begin{minipage}[b]{4em}
{\small
\rotatebox{90}{\hspace{2mm}input}\\
}
\end{minipage}\hspace{-10mm}%
\includegraphics[width=0.1286\textwidth]{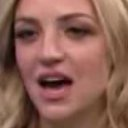}
\hspace{0.0040\textwidth}
\begin{minipage}[b]{4em}
{\small
\rotatebox{90}{\hspace{-3mm}reconstruction}\\
}
\end{minipage}\hspace{-10mm}%
\includegraphics[width=0.129\textwidth]{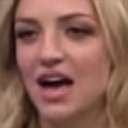}
\includegraphics[width=0.129\textwidth]{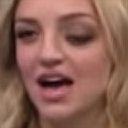}
\includegraphics[width=0.129\textwidth]{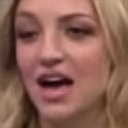}
\includegraphics[width=0.129\textwidth]{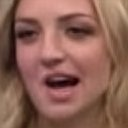}
\includegraphics[width=0.129\textwidth]{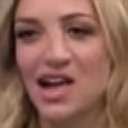}
\includegraphics[width=0.129\textwidth]{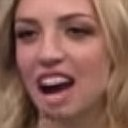}
\\
\hspace*{1.0000em}
\hspace{0.1100\textwidth}
\hspace*{1.0000em}
{\small
\begin{tabu} to 0.84\textwidth{X[c] X[c] X[c] X[c] X[c] X[c]}
\vspace{-3.5000mm}original & \vspace{-3.5000mm}eye down & \vspace{-3.5000mm}eyebrow up & \vspace{-3.5000mm}mouth to side & \vspace{-3.5000mm}nose to side & \vspace{-3.5000mm}open mouth
\end{tabu}
}
\vspace{-5.0000mm}
\end{minipage}
\begin{minipage}{\textwidth}
\begin{minipage}[b]{4em}
{\small
\rotatebox{90}{\hspace{0mm}}\\
}
\end{minipage}\hspace{-10mm}%
\hspace{0.1286\textwidth}
\hspace{0.0040\textwidth}
\begin{minipage}[b]{4em}
{\small
\rotatebox{90}{\hspace{-4mm}manip. keypoints}\\
}
\end{minipage}\hspace{-10mm}%
\includegraphics[width=0.129\textwidth]{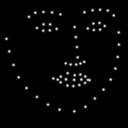}
\includegraphics[width=0.129\textwidth]{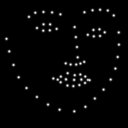}
\includegraphics[width=0.129\textwidth]{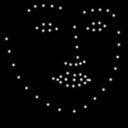}
\includegraphics[width=0.129\textwidth]{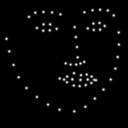}
\includegraphics[width=0.129\textwidth]{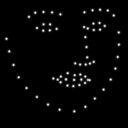}
\includegraphics[width=0.129\textwidth]{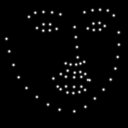}
\\
\begin{minipage}[b]{4em}
{\small
\rotatebox{90}{\hspace{2mm}input}\\
}
\end{minipage}\hspace{-10mm}%
\includegraphics[width=0.1286\textwidth]{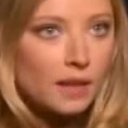}
\hspace{0.0040\textwidth}
\begin{minipage}[b]{4em}
{\small
\rotatebox{90}{\hspace{-3mm}reconstruction}\\
}
\end{minipage}\hspace{-10mm}%
\includegraphics[width=0.129\textwidth]{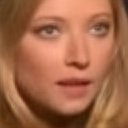}
\includegraphics[width=0.129\textwidth]{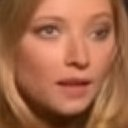}
\includegraphics[width=0.129\textwidth]{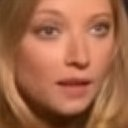}
\includegraphics[width=0.129\textwidth]{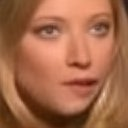}
\includegraphics[width=0.129\textwidth]{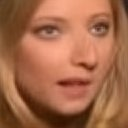}
\includegraphics[width=0.129\textwidth]{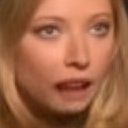}
\\
\hspace*{1.0000em}
\hspace{0.1100\textwidth}
\hspace*{1.0000em}
{\small
\begin{tabu} to 0.84\textwidth{X[c] X[c] X[c] X[c] X[c] X[c]}
\vspace{-3.5000mm}original & \vspace{-3.5000mm}eye down & \vspace{-3.5000mm}eyebrow up & \vspace{-3.5000mm}mouth to side & \vspace{-3.5000mm}nose to side & \vspace{-3.5000mm}open mouth
\end{tabu}
}
\vspace{-5.0000mm}
\end{minipage}
\begin{minipage}{\textwidth}
\begin{minipage}[b]{4em}
{\small
\rotatebox{90}{\hspace{0mm}}\\
}
\end{minipage}\hspace{-10mm}%
\hspace{0.1286\textwidth}
\hspace{0.0040\textwidth}
\begin{minipage}[b]{4em}
{\small
\rotatebox{90}{\hspace{-4mm}manip. keypoints}\\
}
\end{minipage}\hspace{-10mm}%
\includegraphics[width=0.129\textwidth]{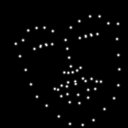}
\includegraphics[width=0.129\textwidth]{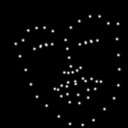}
\includegraphics[width=0.129\textwidth]{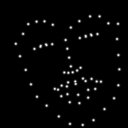}
\includegraphics[width=0.129\textwidth]{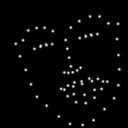}
\includegraphics[width=0.129\textwidth]{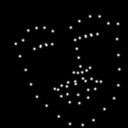}
\includegraphics[width=0.129\textwidth]{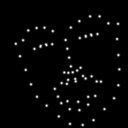}
\\
\begin{minipage}[b]{4em}
{\small
\rotatebox{90}{\hspace{2mm}input}\\
}
\end{minipage}\hspace{-10mm}%
\includegraphics[width=0.1286\textwidth]{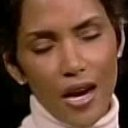}
\hspace{0.0040\textwidth}
\begin{minipage}[b]{4em}
{\small
\rotatebox{90}{\hspace{-3mm}reconstruction}\\
}
\end{minipage}\hspace{-10mm}%
\includegraphics[width=0.129\textwidth]{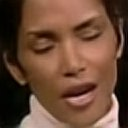}
\includegraphics[width=0.129\textwidth]{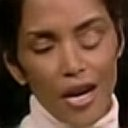}
\includegraphics[width=0.129\textwidth]{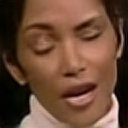}
\includegraphics[width=0.129\textwidth]{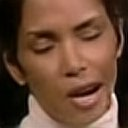}
\includegraphics[width=0.129\textwidth]{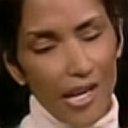}
\includegraphics[width=0.129\textwidth]{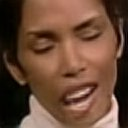}
\\
\hspace*{1.0000em}
\hspace{0.1100\textwidth}
\hspace*{1.0000em}
{\small
\begin{tabu} to 0.84\textwidth{X[c] X[c] X[c] X[c] X[c] X[c]}
\vspace{-3.5000mm}original & \vspace{-3.5000mm}eye down & \vspace{-3.5000mm}eyebrow up & \vspace{-3.5000mm}mouth to side & \vspace{-3.5000mm}nose to side & \vspace{-3.5000mm}open mouth
\end{tabu}
}
\vspace{-5.0000mm}
\end{minipage}
\begin{minipage}{\textwidth}
\begin{minipage}[b]{4em}
{\small
\rotatebox{90}{\hspace{0mm}}\\
}
\end{minipage}\hspace{-10mm}%
\hspace{0.1286\textwidth}
\hspace{0.0040\textwidth}
\begin{minipage}[b]{4em}
{\small
\rotatebox{90}{\hspace{-4mm}manip. keypoints}\\
}
\end{minipage}\hspace{-10mm}%
\includegraphics[width=0.129\textwidth]{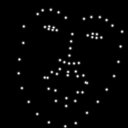}
\includegraphics[width=0.129\textwidth]{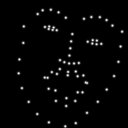}
\includegraphics[width=0.129\textwidth]{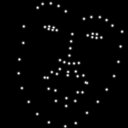}
\includegraphics[width=0.129\textwidth]{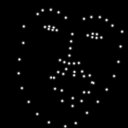}
\includegraphics[width=0.129\textwidth]{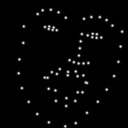}
\includegraphics[width=0.129\textwidth]{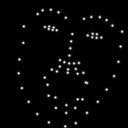}
\\
\begin{minipage}[b]{4em}
{\small
\rotatebox{90}{\hspace{2mm}input}\\
}
\end{minipage}\hspace{-10mm}%
\includegraphics[width=0.1286\textwidth]{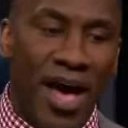}
\hspace{0.0040\textwidth}
\begin{minipage}[b]{4em}
{\small
\rotatebox{90}{\hspace{-3mm}reconstruction}\\
}
\end{minipage}\hspace{-10mm}%
\includegraphics[width=0.129\textwidth]{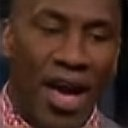}
\includegraphics[width=0.129\textwidth]{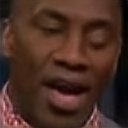}
\includegraphics[width=0.129\textwidth]{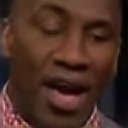}
\includegraphics[width=0.129\textwidth]{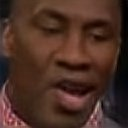}
\includegraphics[width=0.129\textwidth]{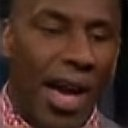}
\includegraphics[width=0.129\textwidth]{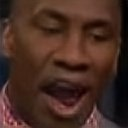}
\\
\hspace*{1.0000em}
\hspace{0.1100\textwidth}
\hspace*{1.0000em}
{\small
\begin{tabu} to 0.84\textwidth{X[c] X[c] X[c] X[c] X[c] X[c]}
\vspace{-3.5000mm}original & \vspace{-3.5000mm}eye down & \vspace{-3.5000mm}eyebrow up & \vspace{-3.5000mm}mouth to side & \vspace{-3.5000mm}nose to side & \vspace{-3.5000mm}open mouth
\end{tabu}
}
\vspace{0.0000mm}
\end{minipage}
